# Supplementary material for: Balancing Multi-Target Semi-Supervised Medical Image Segmentation with Collaborative Generalist and Specialists
Source: arXiv:2504.00862 source file (2025-04-01)
Supplement: Supplementary file 1 [file X_suppl.tex]

\setcounter{page}{1}
% \maketitlesupplementary

\setcounter{section}{0}
In this paper, we propose to collaboratively train a Generalist and Specialists (CGS) to mitigate the issue of scale imbalance in multi-target Semi-Supervised Medical Image Segmentation (SSMIS). In the following sections, we provide details about the analysis of how CGS alleviates scale imbalance (Sec.~\ref{sec:a}) as well as the limitations and future work (Sec.~\ref{sec:b}). In addition to this appendix, we have submitted the code of CGS as the other part of the supplementary material.
\section{Details about Mitigating Scale Imbalance}
\label{sec:a}
In a segmentation task involving $K$ target classes, it is presumed that the individual proportions of these $K$ target classes within the foreground are denoted as $p_i$:
$$p_i = \frac{\sum_{y \in Y} \mathbbm{1}(y = i)}{\sum_{y \in Y} \mathbbm{1}(y \neq 0)},$$ where $i=1,2,...,K$ and $Y$ is the ground truth pixel labels of each image.  
Therefore, $p_i$ should satisfy the following condition: $$p_1 + p_2 + ... + p_K = 1.$$ Conventional approaches depict the participation of each class at the pixel level as $p_1, p_2, ..., p_K$. This leads to a scale imbalance caused by differences between $p_i$ and $p_j$, where $i, j = 1, 2, ..., K$, and $i \neq j$.

In the proposed Multi-Head Specialized Branch, the $i$-th target participates as the \textbf{rest classes} in the training of the remaining $K-1$ classes. More specifically, the participation ratio of the $j$-th class as the \textbf{rest classes} in training is denoted by $1-p_j$. Therefore, it can be deduced that under our framework, the proportion of the $i$-th target participating in the training within the $j$-th specialized segmentation head, $P[i,j]$, is:
$$
P[i,j] = 
\begin{cases}
    p_i & \text{if } i=j \\
    1-p_j & \text{otherwise}
\end{cases}
$$

The total proportion of the $i$-th class $p_i'$ participating in training in our method is obtained as:

$$
p_i'=\frac{\sum_{s=1}^KP[i,s]}{\sum_{s=1}^K\sum_{t=1}^KP[s,t]}
$$

$$
\Rightarrow p_i'= \frac{2p_i+K-2}{K(K-2)+2}
$$
$$
\Rightarrow p_i'- \frac{1}{K}= \frac{2p_iK-2}{K(K(K-2)+2)}
$$
$$
\Rightarrow p_i'- \frac{1}{K}= \frac{2}{(K(K-2)+2)}(p_i-\frac{1}{K}).
$$
When $p_i \neq \frac{1}{K}$:
$$
\frac{|p_i'- \frac{1}{K}|}{|p_i-\frac{1}{K}|}= \frac{2}{(K(K-2)+2)} < 1.
$$
$$
\Rightarrow |p_i'- \frac{1}{K}| < |p_i-\frac{1}{K}|.
$$
When $p_i = \frac{1}{K}$:
$$
    p'_i = p_i = \frac{1}{K}.
$$
In summary, $$|p_i'- \frac{1}{K}| \leq |p_i-\frac{1}{K}|,$$ if and only if $p_i=\frac{1}{K},$ the equation holds true.

Note that, $p_i- \frac{1}{K}$ and $p_i'- \frac{1}{K}$ share the same sign (positive/negative). $|p_i- \frac{1}{K}|$ and $|p_i'- \frac{1}{K}|$ represent the distance between the scale proportion of the $i$-th class and the mean value.

Based on the preceding derivation, it is evident that our proposed training strategy brings the proportion of each class within the foreground closer to the average, thereby effectively mitigating the problem of scale imbalance.

\section{Limitations and Future Work}
\label{sec:b}
In this section, we would like to discuss the limitations of the current CGS as well as the possible ways to further improve it. Firstly, our method is exclusively designed for tasks featuring three or more segmentation targets. When the number of target categories is two, our method reduces to having only one class within the rest classes. Secondly, when there are a particularly large number of categories participating in training, our method might incur high training costs. Fortunately, in the realm of medical imaging, there isn't an overwhelming abundance of targets necessitating segmentation. Thirdly, our proposed CGS is primarily tailored for segmentation tasks involving 2D slices. As detailed in Sec. 4.4, our method can be integrated as a plugin into existing SSMIS methods. Therefore, there is a possibility that our approach could effectively operate within 3D SSMIS methods. We will investigate this issue in future work.
